# Supplementary material for: Combined time and frequency spectroscopy with engineered dual comb spectrometer
Source: arXiv:2212.01687 source file (2022-12-03)
Supplement: Supplementary file 1 [file supp_3.pdf]

# Supplementary material for "Combined time and frequency spectroscopy with engineered dual comb spectrometer"

Sutapa Ghosh and Gadi Eisenstein
*Andrew and Erna Viterby Department of Electrical Engineering and Russell Berrie Nanotechnology Institute, Technion-Israel Institute of Technology, Haifa 32000, Israel*

# I. TWO-DIMENSIONAL SPECTROSCOPY WITH MODULATED DUAL-COMB SPECTROSCOPY

This section describes the formalism for modulated dual-comb spectroscopy (DCS). In modulated DCS, pulse train with repetition rate $T_1$ that probes the sample is amplitude modulated with variable width gate pulses. The sample is consequently being probed by different number of pulses. After probing the sample, the modulated pulse train is measured in a multi-0heterodyne scheme with a reference laser operating at the same wavelength but with a slightly different repetition rate $T_2$.

Consider a pulse train with a repetition rate $T_1$, $E_p(t) = \sum_{l=-\infty}^{\infty} E(t - lT_1) = \sum_l A_l e^{i2\pi lt/T_{rep}}$, where $A_l$ are the Fourier components. The Fourier transform of the pulse train is:

$$E_p(f) = \frac{1}{T_{rep}} \sum_l \mathcal{F}[E(t)](f)\delta(f - l/T_{rep})$$

Mixing of the two pulse trains leads to the formation of an interferogram, $S(t) = |E_p^{(1)} + E_p^{(2)}|^2$.

$$\begin{aligned} S(t) &\approx E_p^{(1)}(t)E_p^{*(2)}(t) \\ &= \sum_l \sum_k A_{1l}A_{2k}^* e^{i2\pi t(\frac{l}{T_1} - \frac{k}{T_2})} \end{aligned}$$

For slightly detuned lasers, $l = k$.

$$\begin{aligned} S(t) &= \sum_l A_{1l}A_{2l}^* e^{i2\pi lt(\frac{1}{T_1} - \frac{1}{T_2})} \\ &= \sum_l A_{1l}A_{2l}^* e^{i2\pi lt\delta f_{rep}} \end{aligned}$$

where, $\delta f_{rep} = (\frac{1}{T_1} - \frac{1}{T_2})$

The Fourier transform of the beat interferogram is:

$$S(f) = \frac{1}{T_1 T_2} \sum_l ]\mathcal{F}[E_1(t)](f)\mathcal{F}[E_2^*(t)](f)\delta(f - l\delta f_{rep}) \tag{S1}$$

Once one pulse train passes through an intensity modulator (EOM) driven by $y(t)$, the pulse train, $E_p(t)$ becomes:

$$E_{mod}(t) = y(t)E_p(t)$$

and its Fourier transform is:

$$\begin{aligned} E_{mod}(f) &= \frac{1}{2\pi} \int_{f'=-\infty}^{\infty} df' y(f - f')E_p(f') \\ &= \frac{1}{2\pi T_{rep}} \sum_l y(f - lf_{rep})F(E(t))(lf_{rep}) \end{aligned}$$

The modulation function is periodic with a repetition rate $T$ $y(t) = \sum_m y_0(t - mT)$,

$$y(f) = \frac{1}{T} \sum_m F(y_0)(f)\delta(f - \frac{m}{T})$$

$$E_{mod}(f) = \frac{1}{2\pi T_{rep} T} \sum_l \sum_m F(y_0)(f - lf_{rep})F(E(t))(lf_{rep})\delta(f - lf_{rep} - \frac{m}{T}) \tag{S2}$$

Wich represents the Fourier transform of the modulated electric field.

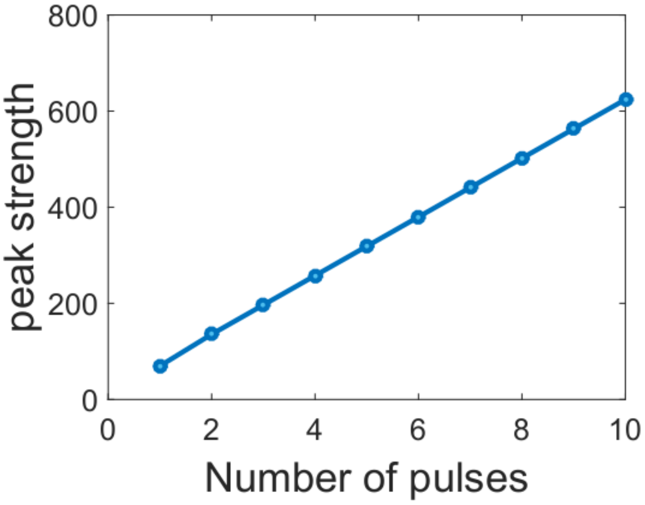


Fig. S1. **Heterodyne signal strength as a function of number of pulses** The beat between the modulated pulse train and reference laser is calculated and the signal strength is plotted as a function of number of pulses in each modulation cycle. It shows a linear dependence.

The intensity modulated pulse train mixes with the reference laser and generates heterodyne beats. The DCS spectrum becomes:

$$\begin{aligned}
E_{mod}(t) &= \frac{1}{2\pi T_1 T}\sum_l\sum_m A^{mod}_{lm} e^{i2\pi t(lf_{rep,1}+mf_{rep})} \\
S(t) &= E_{mod}(t)E^{*(2)}_p(t) \\
&= \frac{1}{2\pi T_1 T T_2}\sum_l\sum_m A^{mod}_{lm} e^{i2\pi t(lf_{rep,1}-mf_{rep})}\sum_k A^*_{2k} e^{-i2\pi kt/T_2} \\
&= \frac{1}{2\pi T_1 T T_2}\sum_l\sum_m\sum_k A^{mod}_{lm} A^*_{2k} e^{i2\pi t(lf_{rep,1}+mf_{rep}-kf_{rep,2})} \\
S(f) &= \frac{1}{2\pi T_1 T T_2}\sum_l\sum_m\sum_k F(y_0)(f-lf_{rep,1})F(E_1)(lf_{rep,1})F(E_2)(f)\delta(f-lf_{rep,1}-mf_{rep}+kf_{rep,2})
\end{aligned}$$

Changing the modulation width allows varying the number of probe pulses in each modulation cycle. With every added pulse, the strength of the beat signal also changes. Fig. S1, shows the effect of modulation width increase on the Fourier signal strength, the dependence is linear.

The modulated laser pulse train passes through the sample before the multi-heterodyne measurement. The sample properties are imprinted on the pulsed signal are are retrieved from the dual-comb spectrogram.

$$S(t) = \frac{1}{2\pi}\sum_l\sum_m\sum_k A^{mod}_{lm} A^*_{2k} e^{i2\pi t(lf_{rep,1}+mf_{rep}-kf_{rep,2})} e^{-\alpha_{lm}-i\phi_{lm}} \quad \text{(S3)}$$

$$S(f) = \frac{1}{2\pi}\sum_l\sum_m\sum_k A^{mod}_{lm} A^*_{2k} e^{-\alpha_{lm}-i\phi_{lm}}\delta(f-lf_{rep,1}-mf_{rep}+kf_{rep,2}) \quad \text{(S4)}$$

The modulated pulse train allows probing the sample with broadband signals along with probing the sample at different times. This generates a two dimensional spectroscopy of a sample. To check the validity of our method, we simulated a sample with a quadratic population dependence on time which we were able to retrieve by calculating the two-dimensional spectroscopy with the modulated DCS method

## II. LIGHT MATTER INTERACTION OF A TWO LEVEL SYSTEM IN MODULATED DCS

This section discusses the interaction of a two-level system with a laser pulse train. Consider a two level system with ground state $|g\rangle$ and excited state $|e\rangle$ separated by $\omega_0$ and interacting with a classical electromagnetic field comprising a train of modulated pulses. The Hamiltonian for this system is $H = H_{atom} + H_{int}$. The atomic Hamiltonian is given by, $H_{atom} = \hbar\omega_0 |e\rangle\langle e| = \hbar\omega_0\sigma^\dagger\sigma$. The interaction Hamiltonian is, $H_{int} = -d.E_{mod}(t) =$

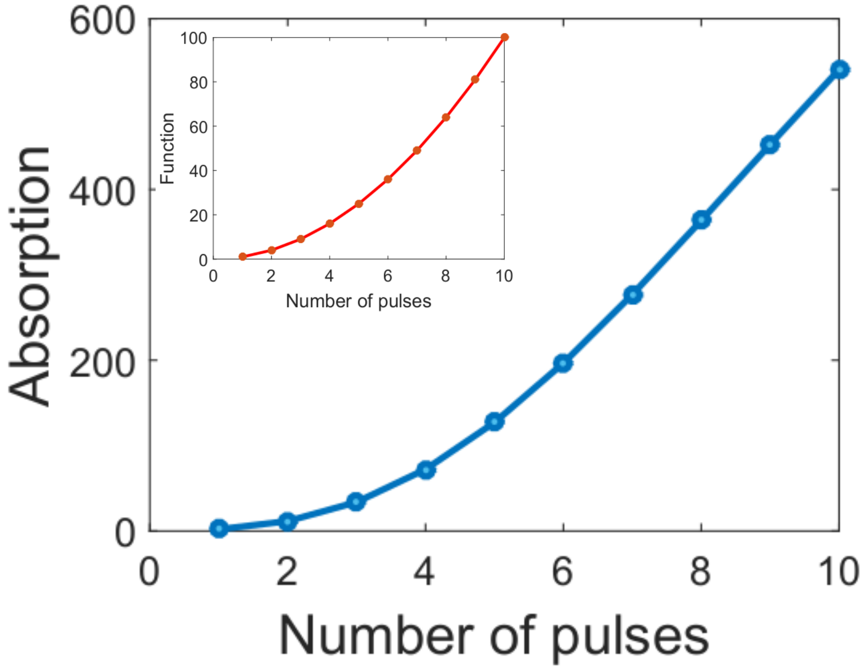


Fig. S2. **Simulated temporal evolution of a sample retrieved from multi-dimensional modulated DCS method.** The absorption spectrum is calculated by changing the number of the pulses interacting with the sample. The multi-dimensional spectrum is calculated which recovers the temporal evolution of the sample. The Inset shows the assumed sample response function with the number of interacting pulse.

$\hbar\Omega(\sigma e^{i\omega t} + \sigma^\dagger e^{-i\omega t})$, where d is the dipole moment corresponding a particular transition, $\Omega = -\frac{\langle g|(\hat{e}.d)|e\rangle E_{mod}}{\hbar}$ is the Rabi frequency.

After interaction with the optical field, the wavefunction of the atoms can be written in terms of eigenvectors as, $|\psi(t)\rangle = \sum_i C_i e^{-iE_0 t/\hbar}|i\rangle$. From the time-dependent Schroedinger equation, we can calculate the Bloch equation in a rotating frame with frequency $\Delta = \omega - \omega_0$

$$\frac{\partial C_g}{\partial t} = -i\Omega(t)\tilde{C}_e \tag{S5}$$

$$\frac{\partial C_e}{\partial t} = i\Delta C_e - i\Omega(t)C_g \tag{S6}$$

The population dynamics of the excited state is calculated by solving the Bloch equation (S5 and S6) for the modulated electric field as a function of the number of interacting pulses, as described in Fig. S2.
